# Supplementary material for: A Multimodal Foundation Agent for Financial Trading: Tool-Augmented, Diversified, and Generalist
Source: arXiv:2402.18485 source file (2024-06-28)
Supplement: Supplementary file 1 [file app_implementation_details.tex]

Although \texttt{FinAgent}'s training and inference can be done without a GPU, we utilized a single NVIDIA RTX A6000 GPU for our benchmark methods. For dataset split, the data from the latter half of the year is allocated for testing (2023-06-01 $\sim$ 2024-01-01) purposes, while the data from the penultimate year is utilized for training (2022-06-01 $\sim$ 2023-06-01). To ensure equitable comparison, all benchmarks are conducted within the same RL environment for both training and evaluation.

\noindent
\textbf{Benchmark Setup.} In the training phase, we use OPTUNA \cite{akiba2019optuna} for hyperparameter optimization, adapting both rule-based and RL methods to trading. This process is followed by an evaluation with the optimal parameters. We employ the officially provided default parameters for both training and testing of FinGPT and FinMem.

\noindent
\textbf{FinAgent Setup.} For each training dataset, we perform only one round of training without the usual requirement for multiple iterations in fine-tuning LLMs. As demonstrated by FinMem \cite{yu2023finmem}, OpenAI's GPT-4 shows improved performance over GPT-3.5. Consequently, we have selected GPT-4 as the foundational LLM for \texttt{FinAgent}. For the market intelligence and decision-making modules, which do not process visual data, we use the \texttt{gpt-4-1106-preview}. In contrast, the two reflection modules, which require an in-depth understanding of visual data, utilize \texttt{gpt-4-vision-preview}. For the memory module, which is designed to store and retrieve texts based on text similarity, a text encoder is essential for vectorizing the text. We adopt \texttt{text-embedding-3-large} for this purpose. The top-k of our retrieval samples is 5. In the low-level reflection module, short term, medium term and long term are for the latest 1 day, 7 days and 14 days respectively. It is important to note that past and future asset price increases and decreases are visible during the training phase, but only past trends are visible during the testing phase to prevent data leakage. The following experiments related to \texttt{FinAgent} all have diversified retrieval if not specifically noted.
